# Supplementary material for: Understanding factors behind IoT privacy -- A user's perspective on RF sensors
Source: arXiv:2401.08037 source file (2024-03-03)
Supplement: Supplementary file 1 [file 8-appendix.tex]

\appendix

\begingroup
    % \fontsize{12pt}{12pt}\selectfont

\section*{Appendix}
% \sectionfont{\fontsize{8}{15}\selectfont}
\section*{Survey Questions}
% \sectionfont{\fontsize{8}{15}\selectfont}

% \chaptertitlefont{\Huge}
% \noindent \chapter{ Survey Questions} \\

\noindent Consent, screening and demographic questions omitted for brevity. \\

\vspace{-0.15in}
\begin{itemize}

    \item[] 
    \item[] Q1. Check all the devices you currently own:
    \begin{itemize}
        \setlength{\itemindent}{-0.3in}
        \item[-] WiFi Router
        \item[-] Laptop Computer
        \item[-] Smartphone
        \item[-] Smart TV
        \item[-] Activity Tracker (e.g. Fitbit or Apple Watch)
        \item[-] Smarthome Hub (e.g., Amazon Echo, Google Alexa)
        \item[-] A car that connects to the internet (e.g., Tesla)
        \item[-] Smart Thermostat (e.g., Nest)
        \item[-] Smart Appliance (e.g., Coffeemaker, Refrigerator, Oven, Fridge)
        \item[-] Smart Door Locks (e.g., Door locks for your home you can open via Bluetooth)
        \item[-] Smart Lighting (e.g., Connected lighting switches, dimmers, or bulbs)
        \item[-] None of the above
    \end{itemize}
    
     % known data from devices
    \item[] 
    \item[] Q2. Please select a sensor and device if you know what kind of information they collect.  Multiple selections are possible:
    \begin{itemize}
        \setlength{\itemindent}{-0.3in}
        \item[-] Camera
        \item[-] Microphone
        \item[-] Radar
        \item[-] WiFi Router
        \item[-] Motion Sensor
        \item[-] Thermal Camera
        \item[-] Intertial Sensors (such as IMU, Accelerometer)
        \item[-] LiDAR
        \item[-] Ultrasonic Sensors
    \end{itemize}

    \begin{figure*}[!tbp]
    
    \centering
          {\subfloat[]{\includegraphics[width=0.1\textwidth]{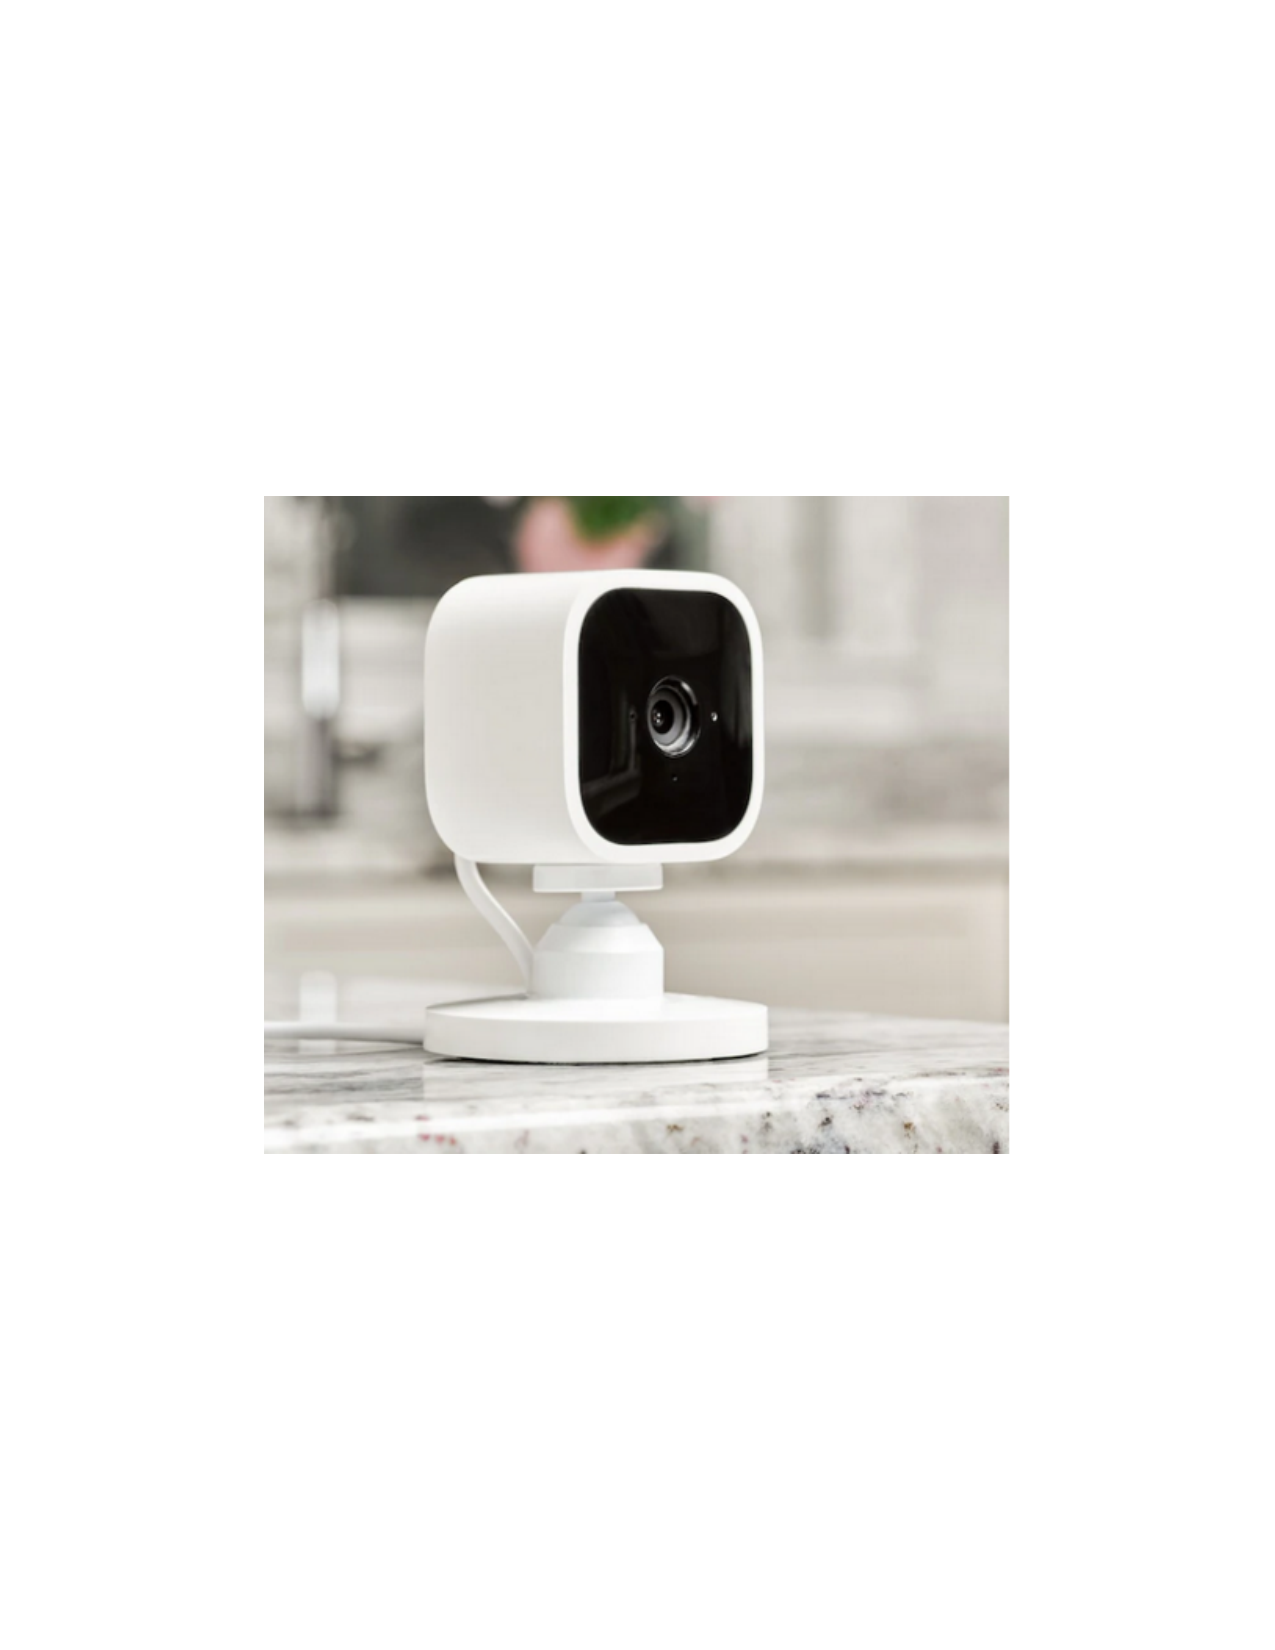}}
          \subfloat[]{\includegraphics[width=0.1\textwidth]{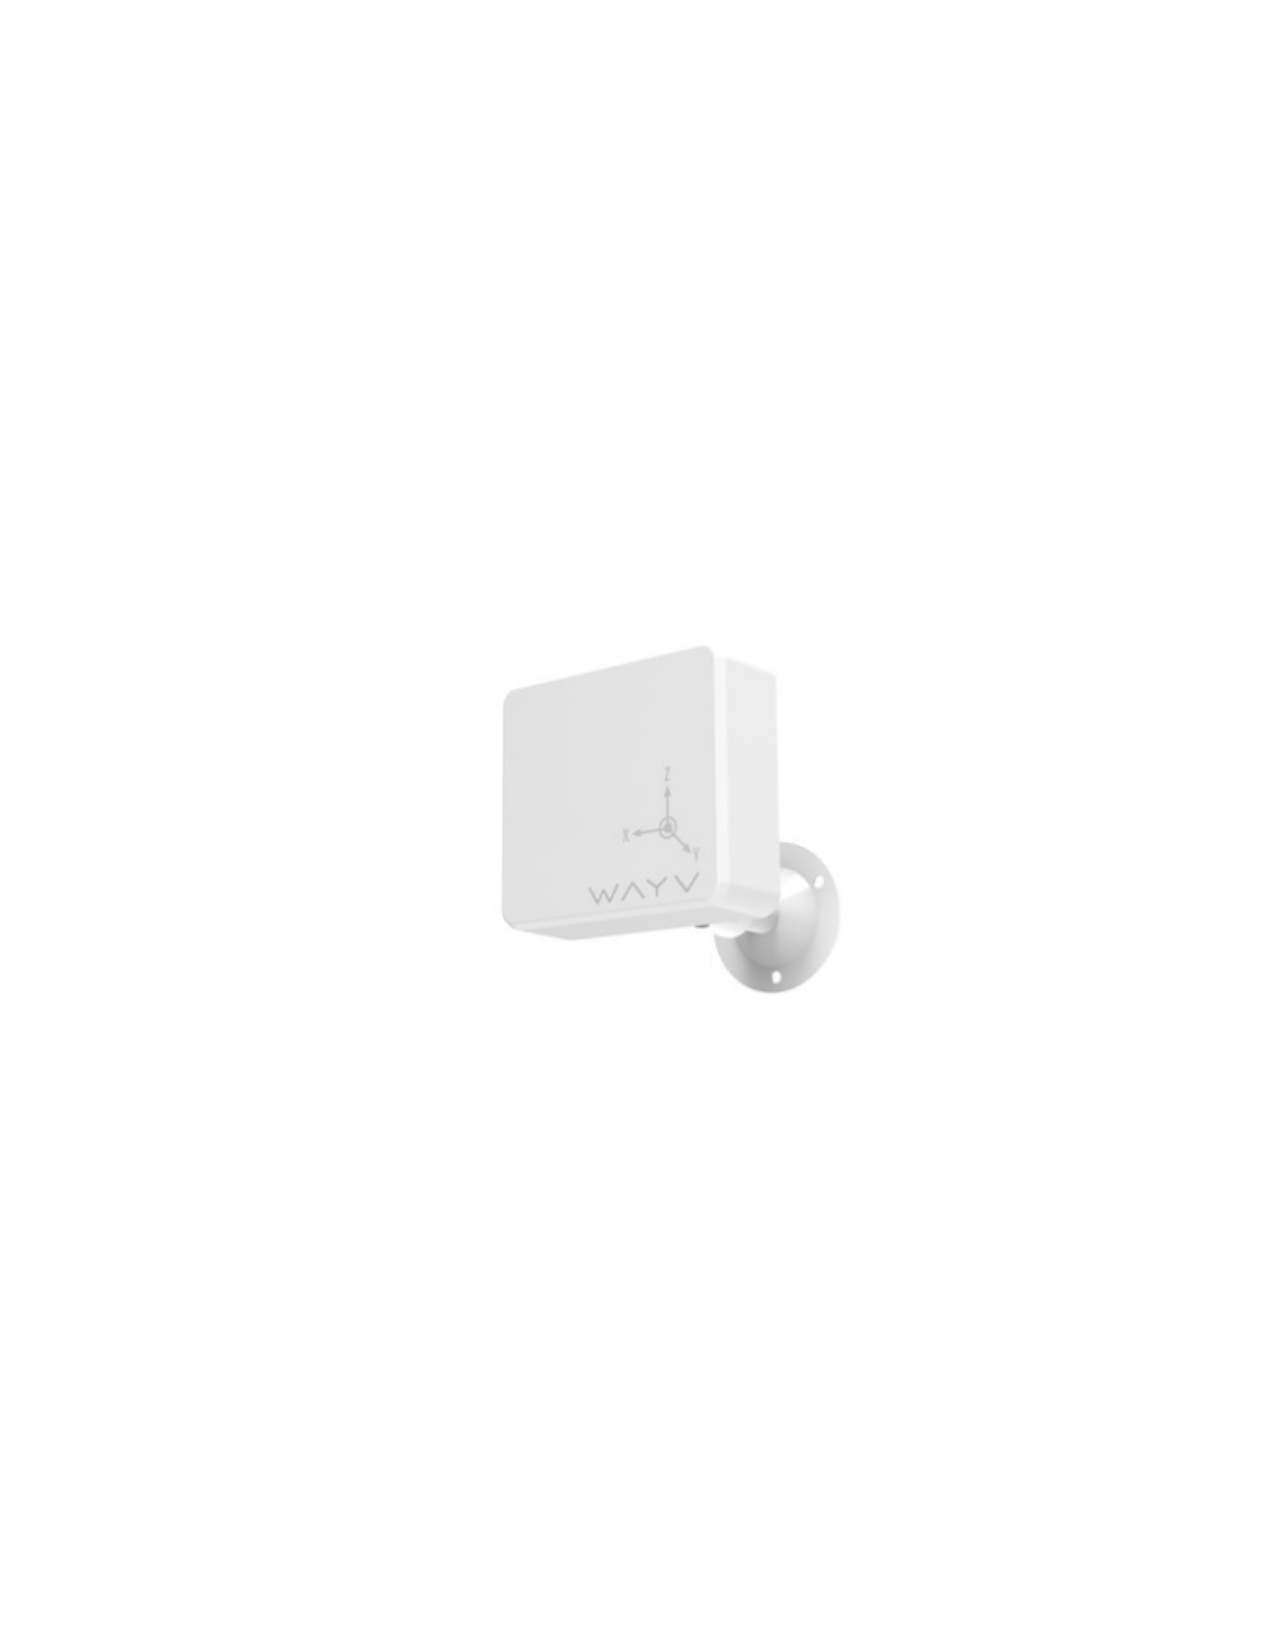}}
          \subfloat[]{\includegraphics[width=0.1\textwidth]{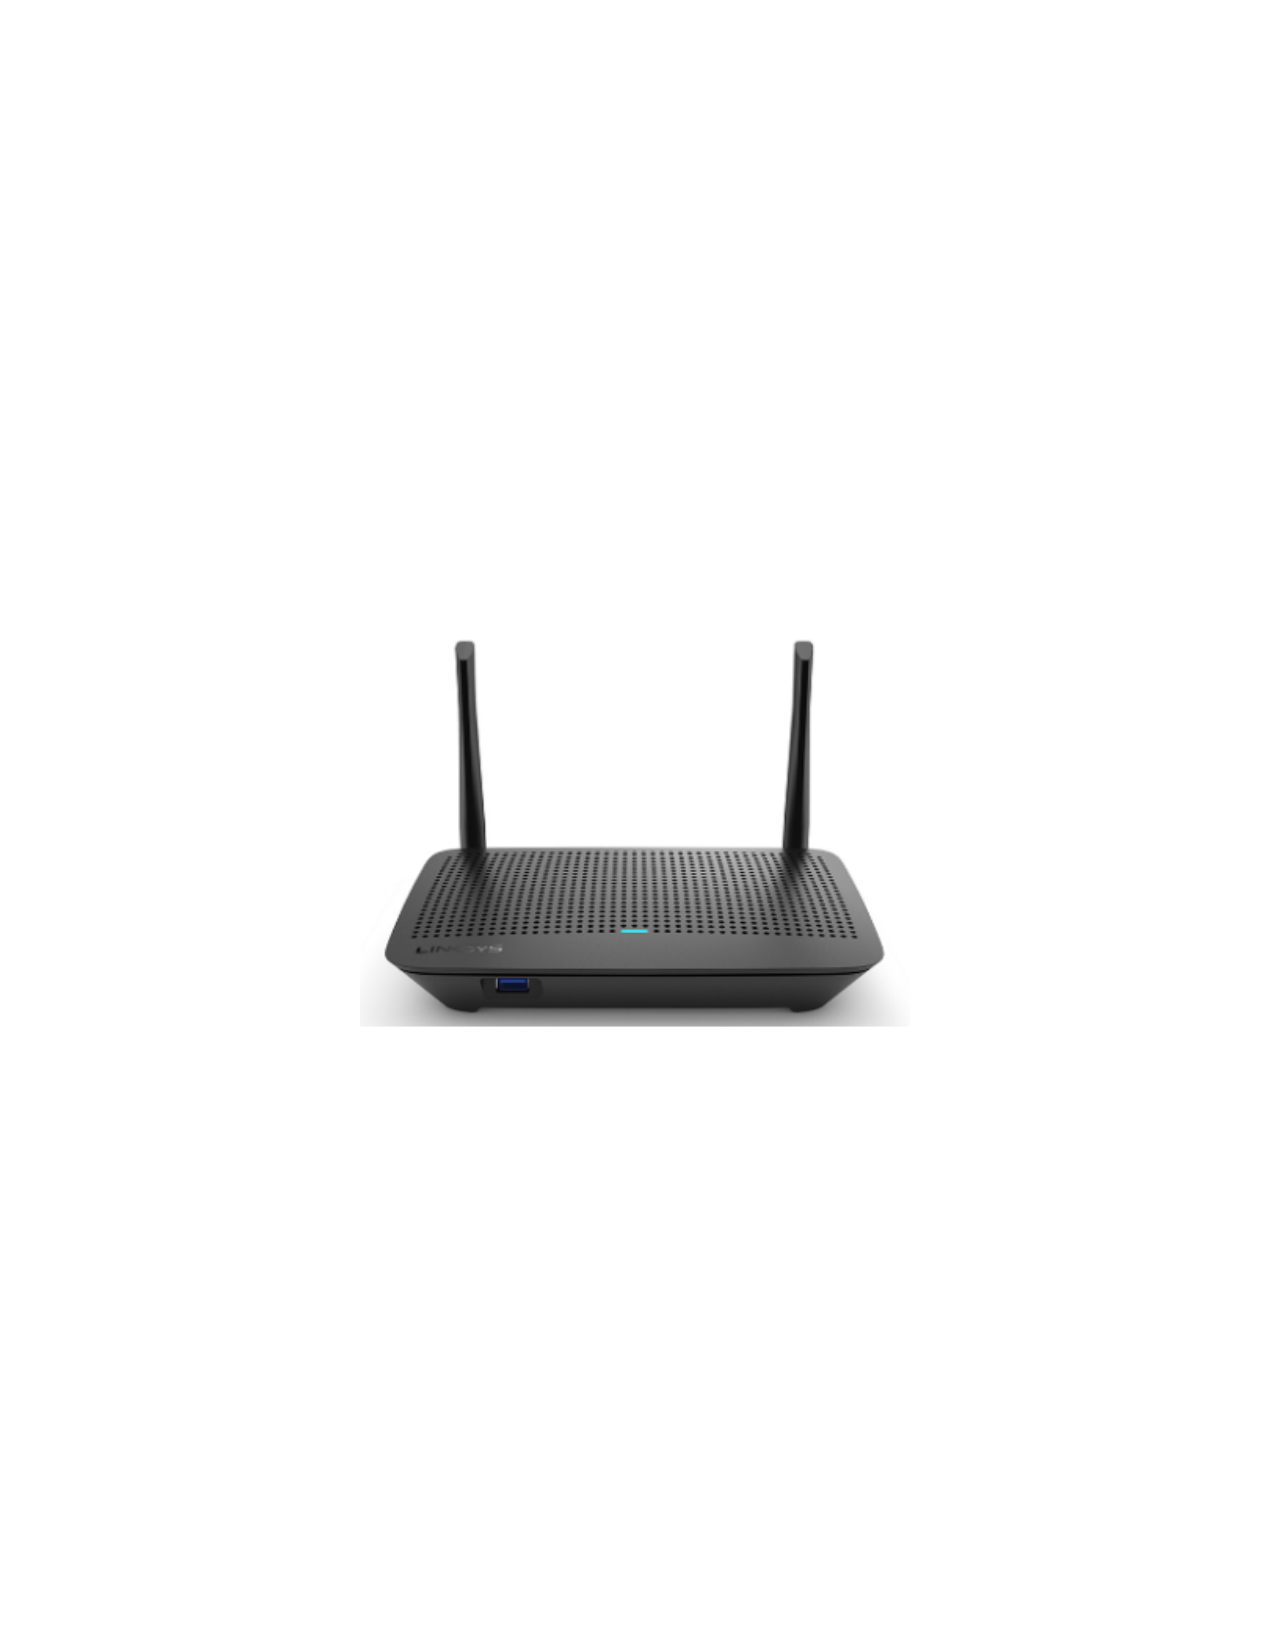}}
          \subfloat[]{\includegraphics[width=0.1\textwidth]{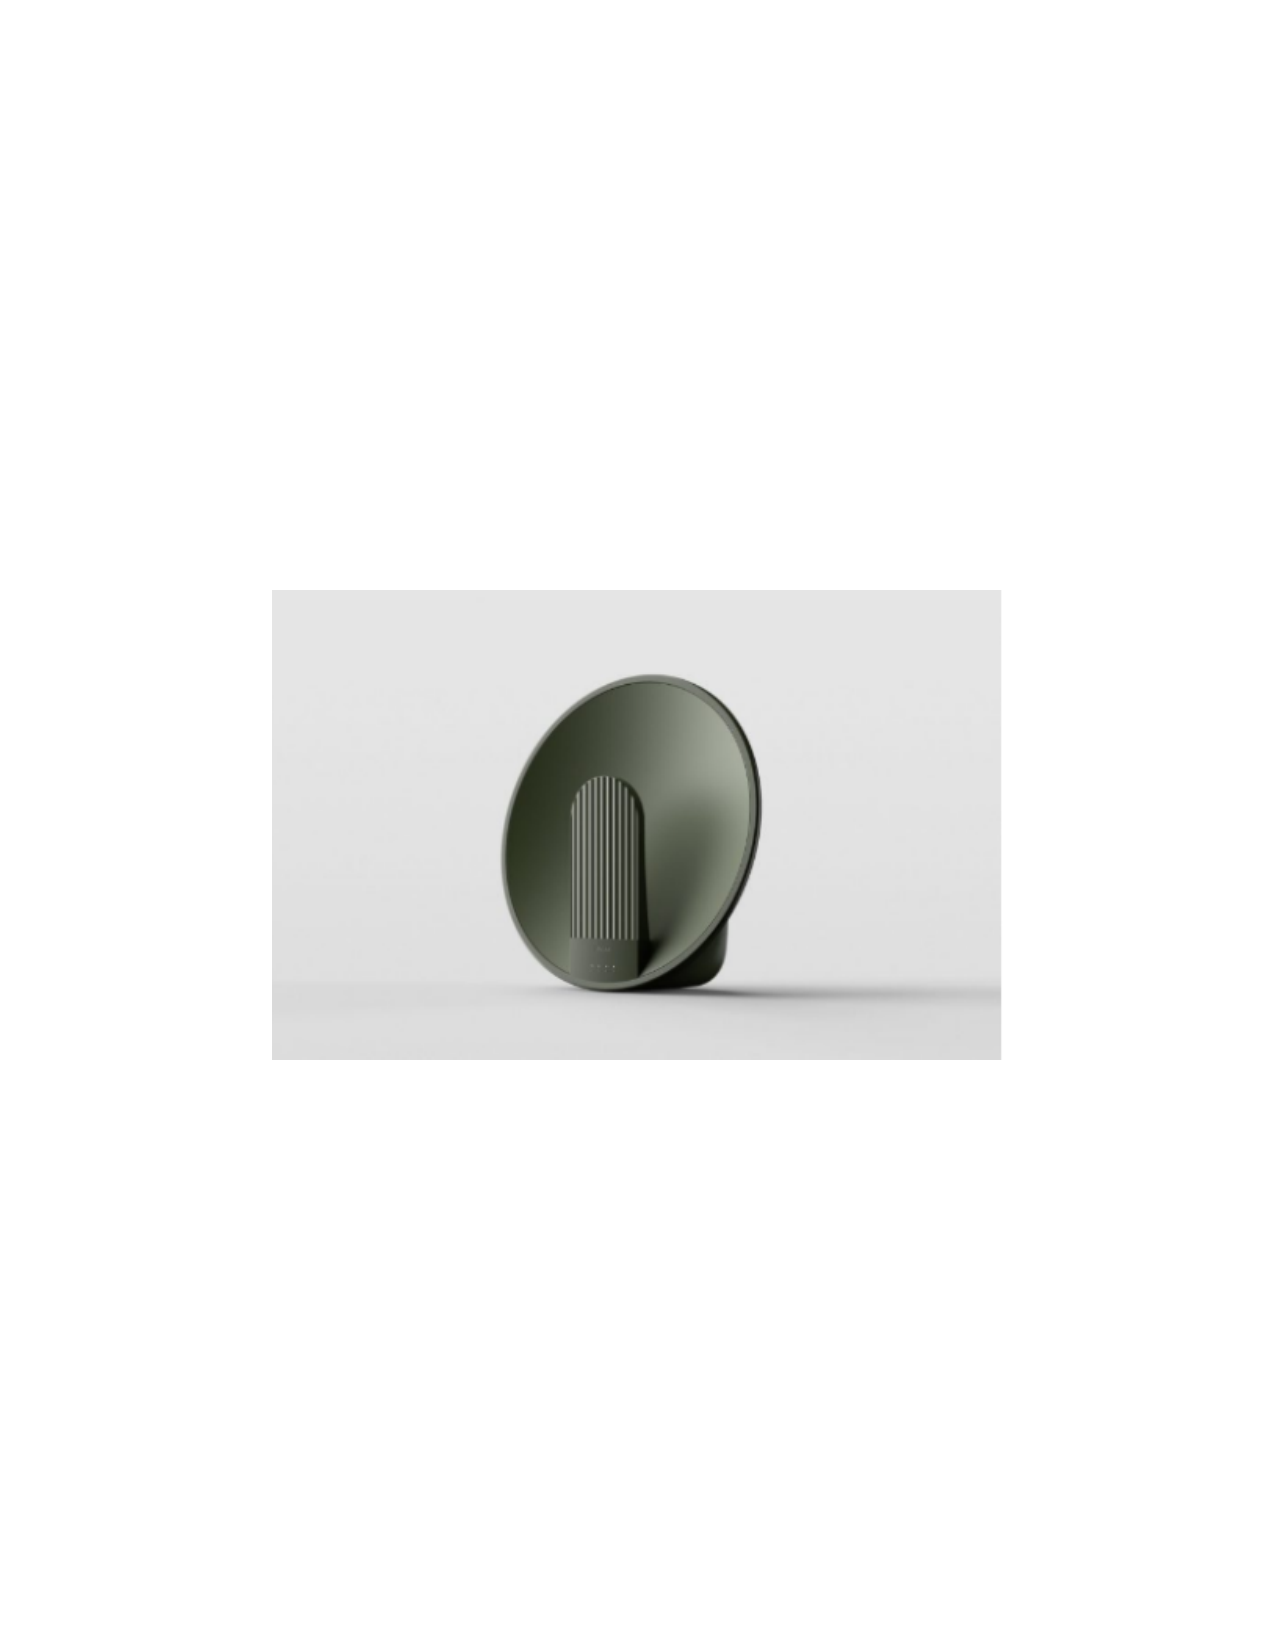}}
          \subfloat[]{\includegraphics[width=0.1\textwidth]{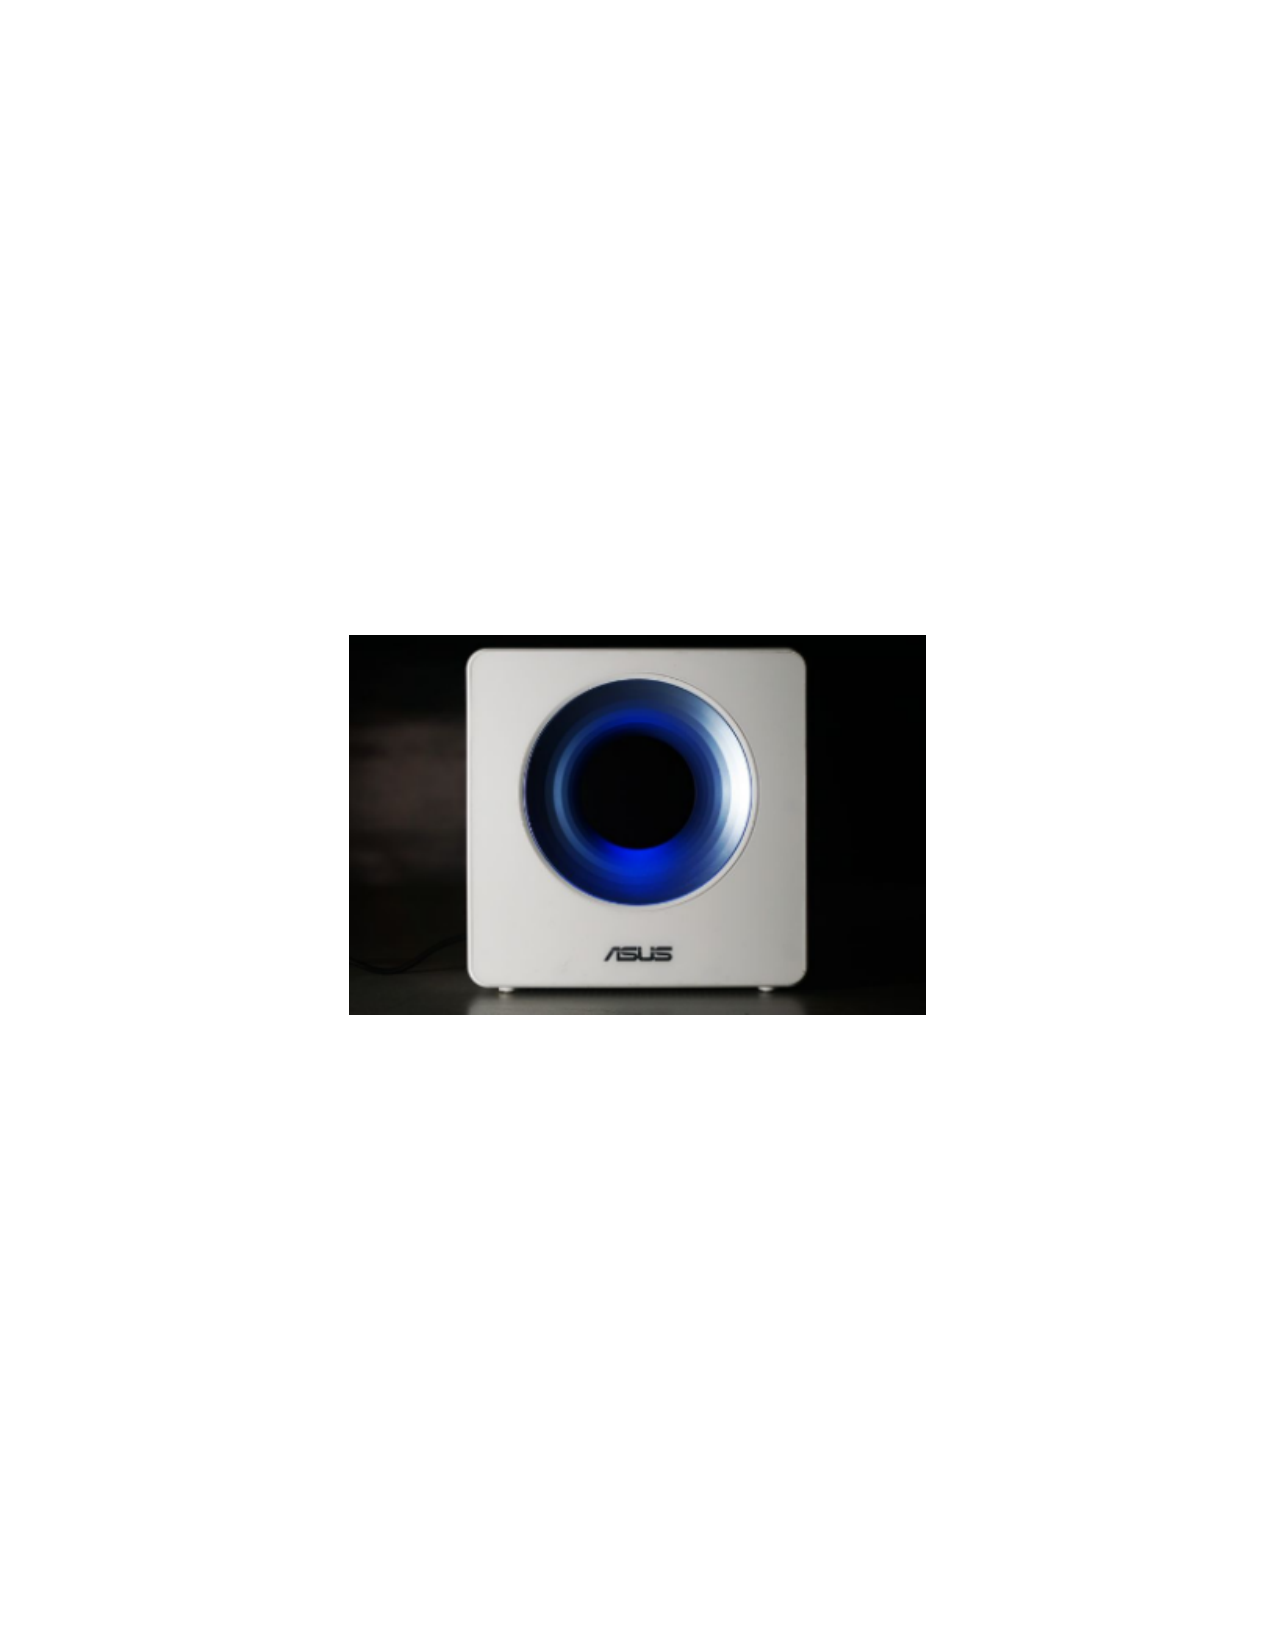}}
          \subfloat[]{\includegraphics[width=0.1\textwidth]{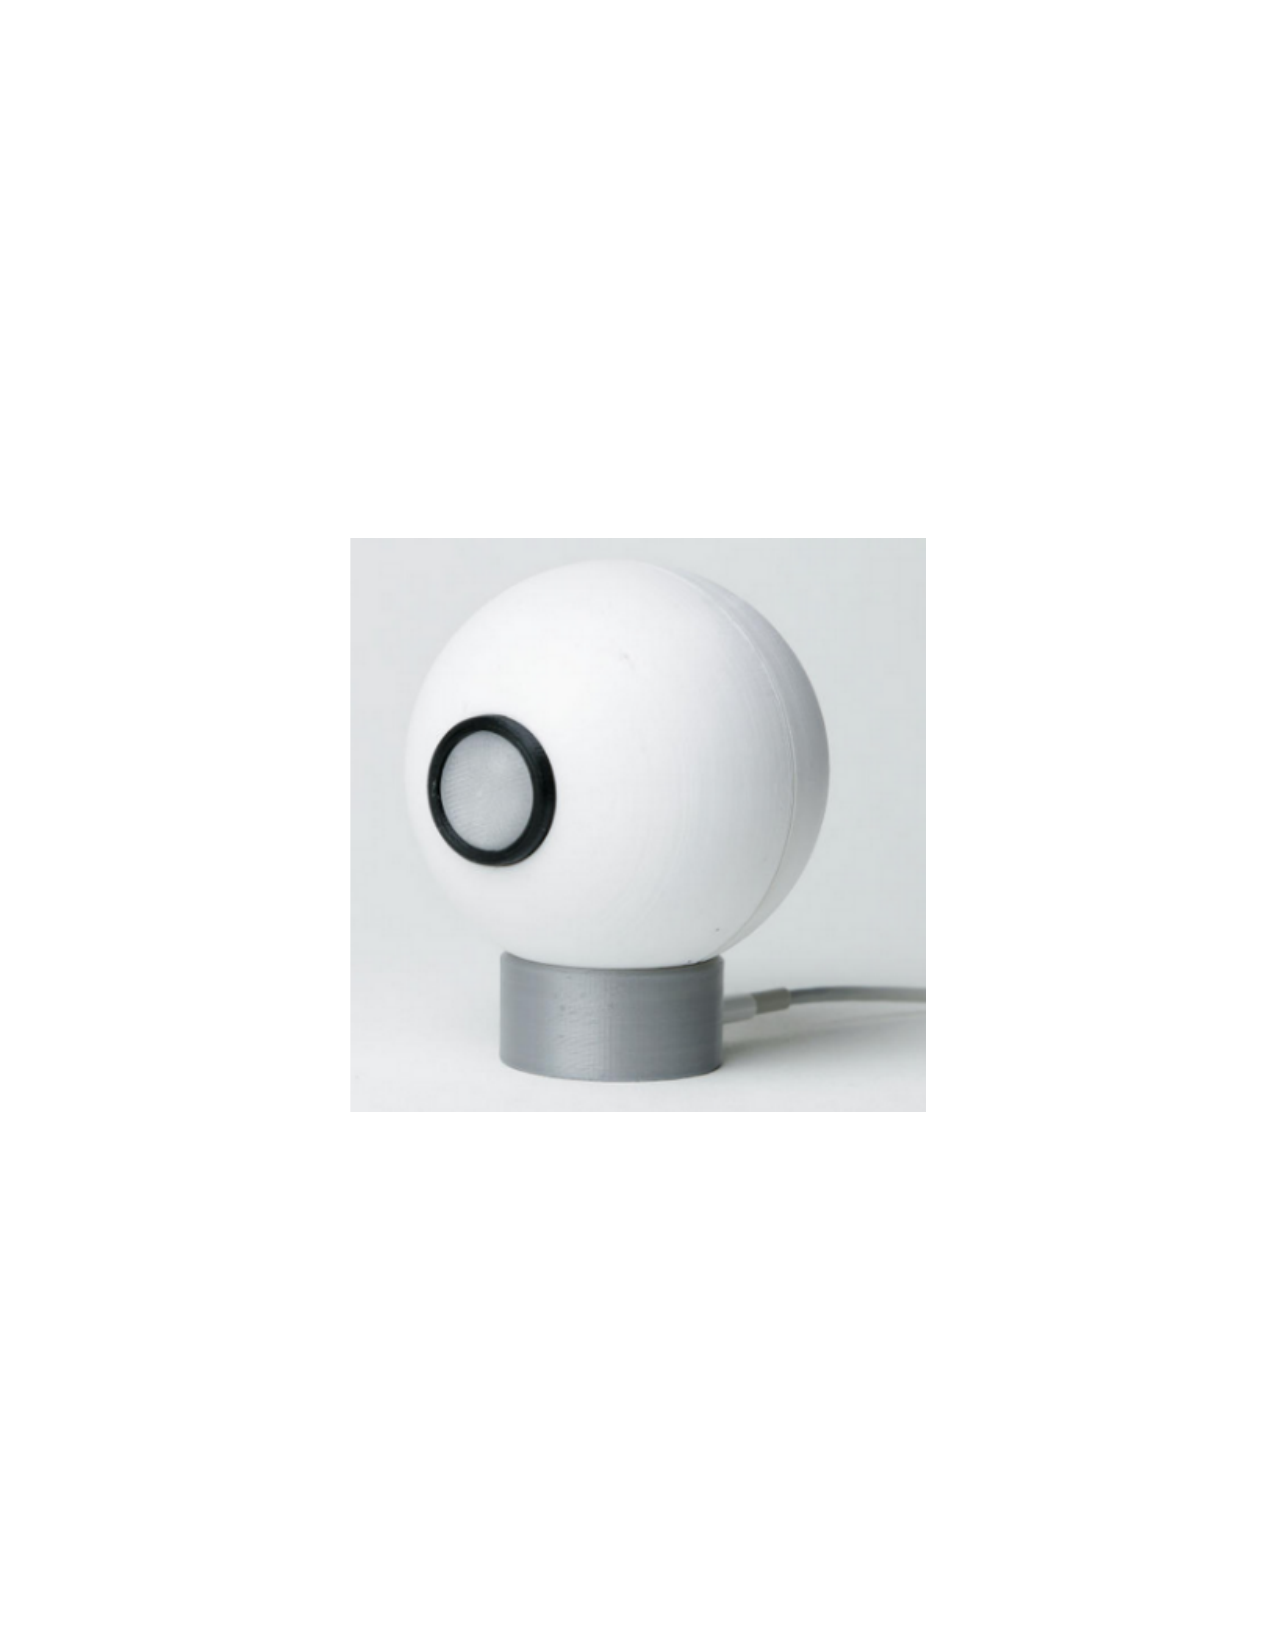}}
          \subfloat[]{\includegraphics[width=0.1\textwidth]{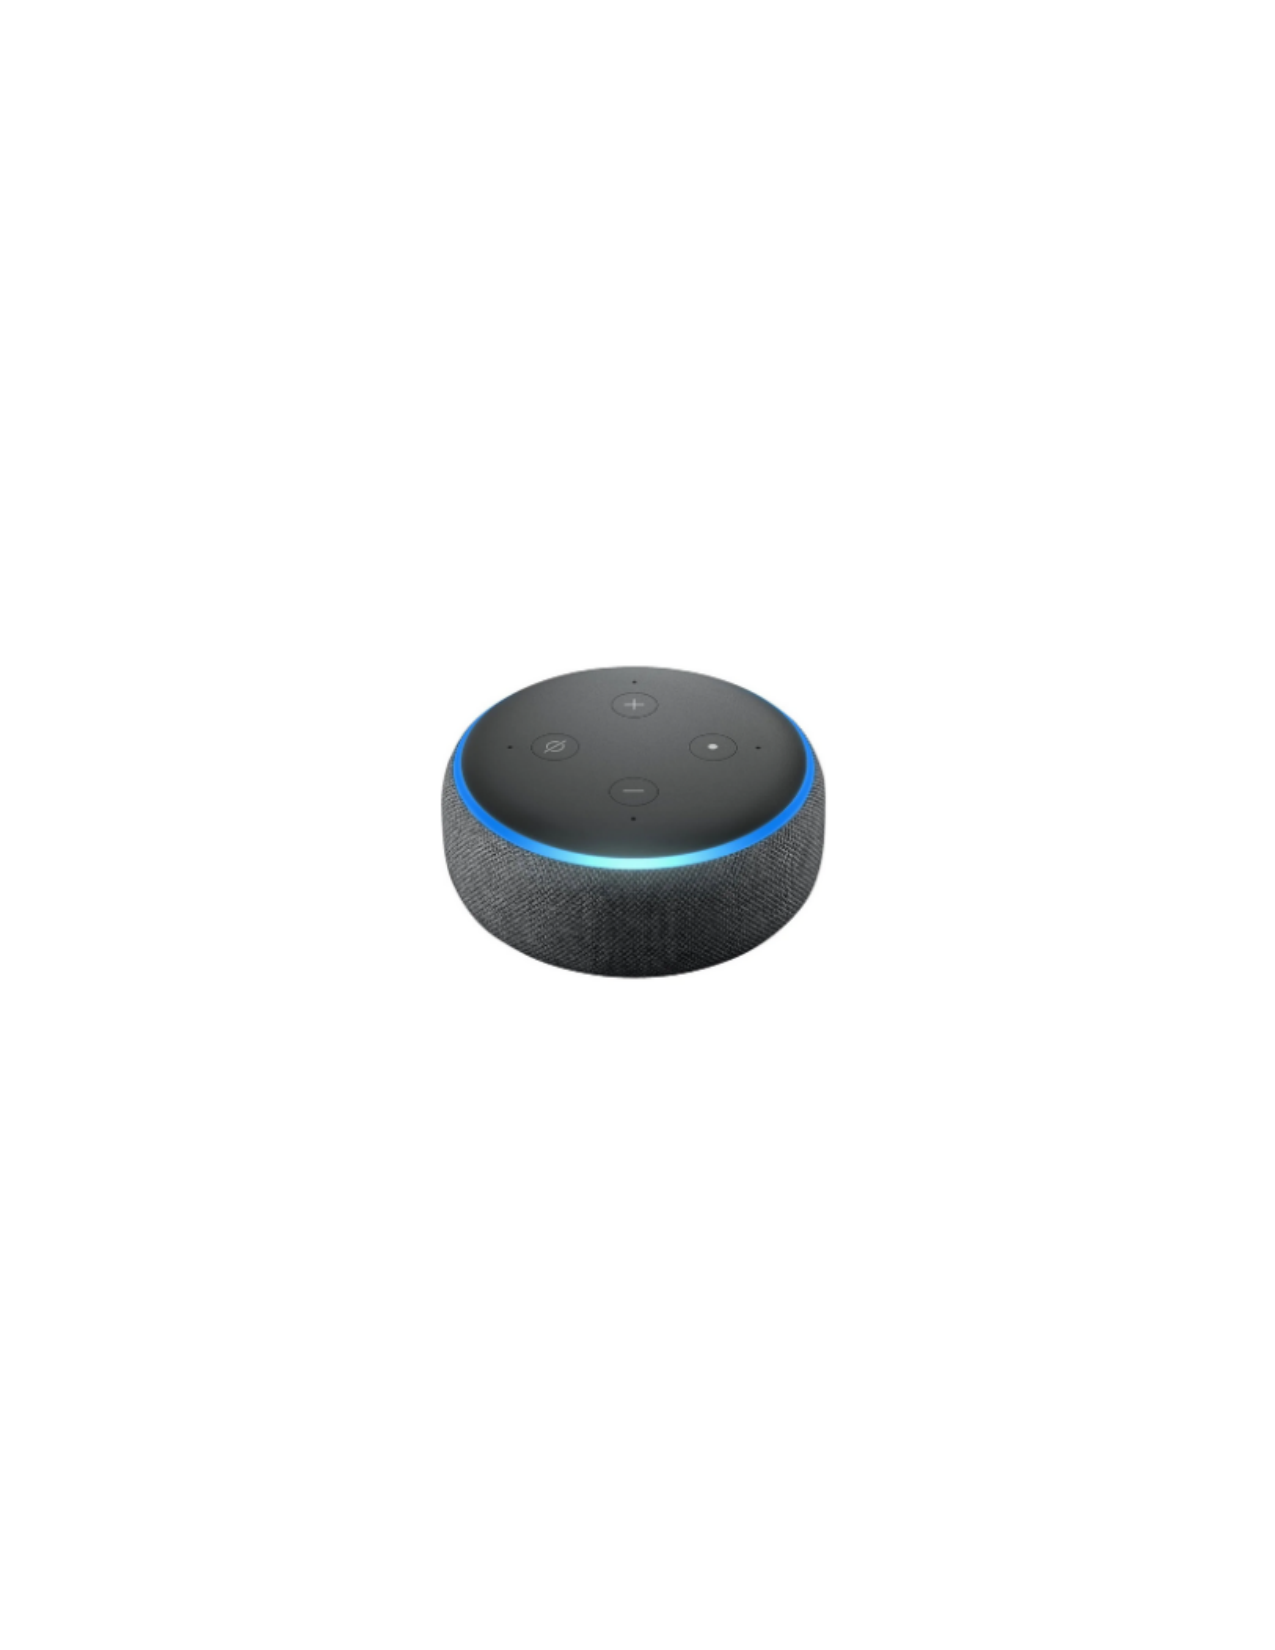}}
          \subfloat[]{\includegraphics[width=0.1\textwidth]{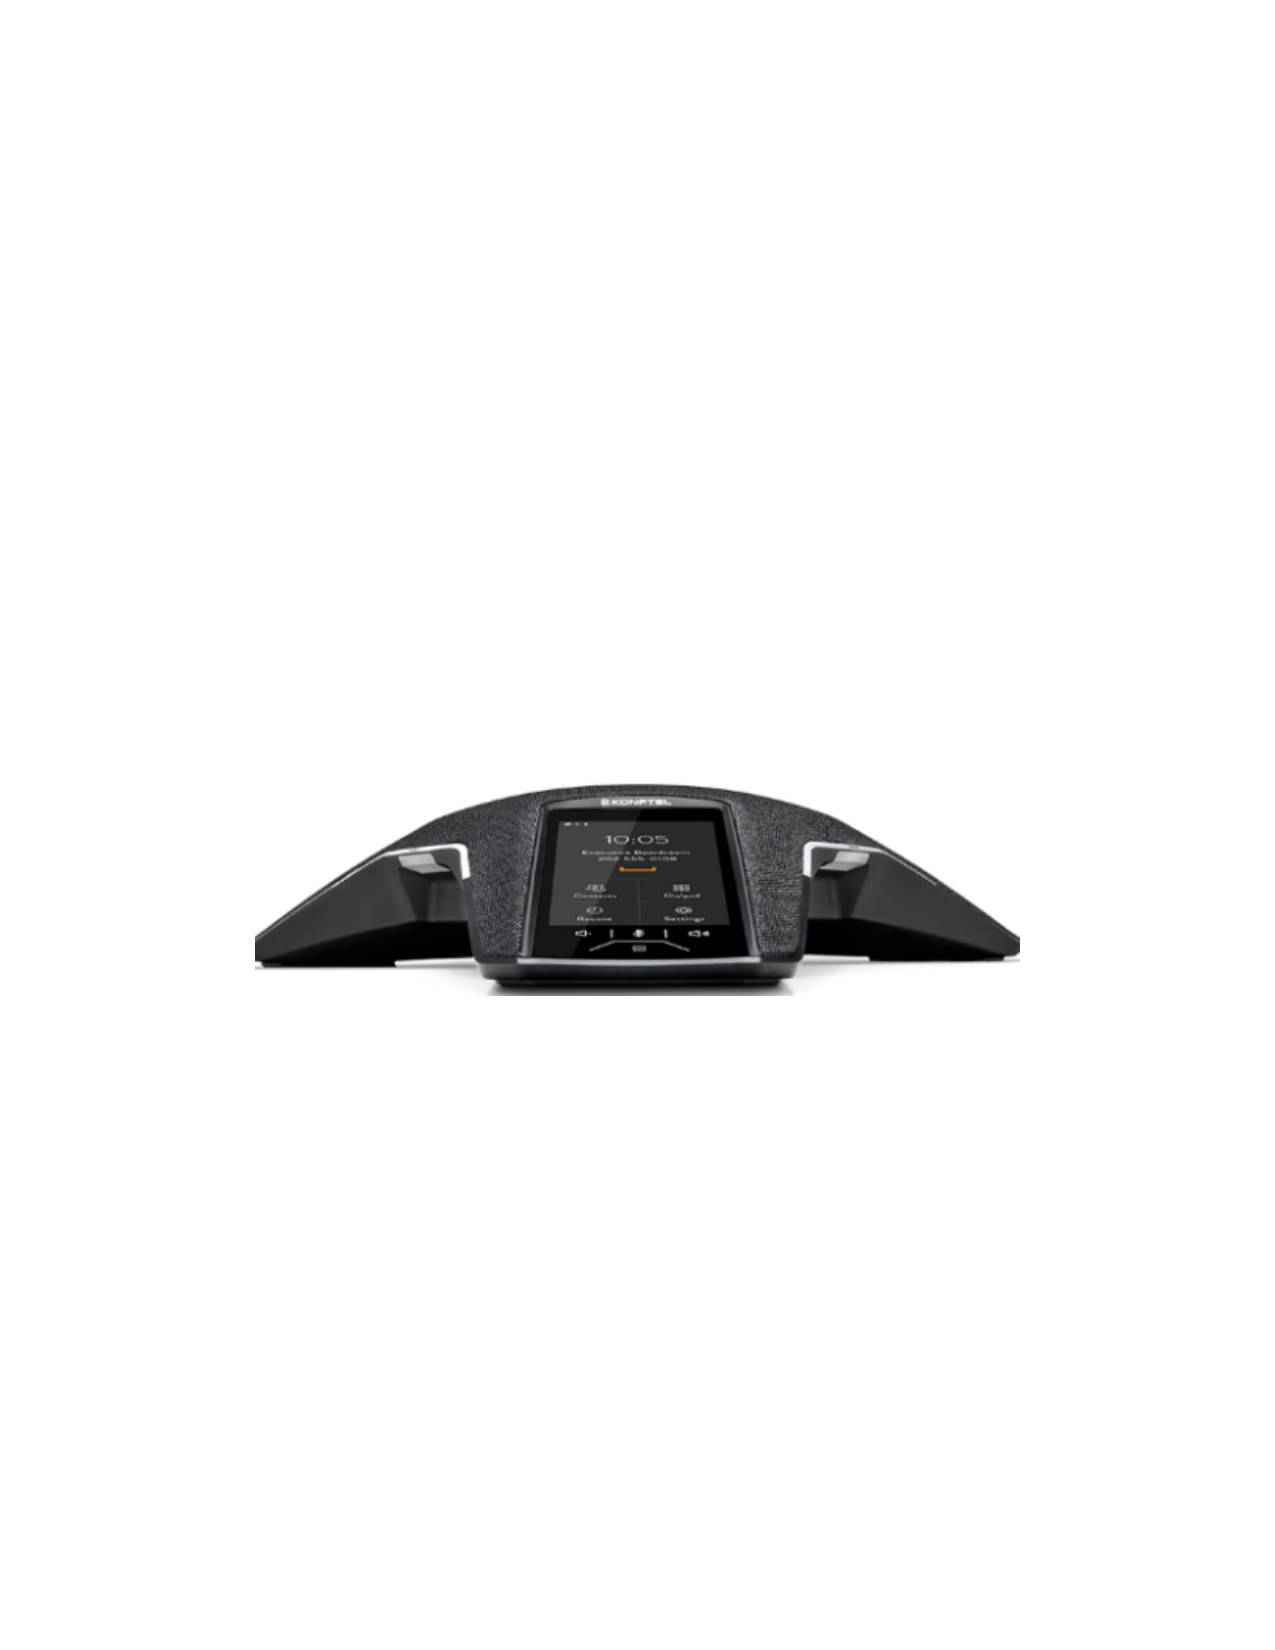}}
            \label{fig:dev1}}
          \hfill
        %   \subfloat[]{\includegraphics[width=0.15\textwidth]{SurveyImages/survey_image2.PNG}
        %     \label{fig:dev2}}
         
        %   \subfloat[]{\includegraphics[width=0.15\textwidth]{SurveyImages/survey_image3.PNG}
        %   \label{fig:dev3}}
        %   \hfill
        %   \subfloat[]{\includegraphics[width=0.15\textwidth]{SurveyImages/survey_image4.PNG}}
          
        % \subfloat[]{\includegraphics[width=0.15\textwidth]{SurveyImages/survey_image5.PNG}}
        %   \hfill
        %   \subfloat[]{\includegraphics[width=0.15\textwidth]{SurveyImages/survey_image6.PNG}}
    
        % \subfloat[]{\includegraphics[width=0.15\textwidth]{SurveyImages/survey_image7.PNG}}
        %   \hfill
        %   \subfloat[]{\includegraphics[width=0.15\textwidth]{SurveyImages/survey_image8.PNG}}
       
        \caption{Sensing Devices used in the survey. L-R (a) Amazon Blink Camera (b) Wayv Air mmWave radar (c) LinkSys WiFi router, (d) Radar router (A WiFi router that looks like a microphone) (e) Asus Blue Cave (A WiFi router that looks like a camera) (f) Maurice Misho camera concept (g) Amazon Echo Dot (h) Konftel Microphone used for video conferencing}
        \label{fig:survey_devices}
    \end{figure*}

    \item[] In the following section, we iterated over a set of devices and asked the same set of questions for each device.
    
    % Familiarity with devices 
    \item[] 
    \item[] Q3/Q6/Q9/Q12/Q15/Q18/Q21/Q24. How familiar are you with the device in \figref{fig:survey_devices}
    \begin{itemize}
        \setlength{\itemindent}{-0.3in}
        \item[-] Very Unfamiliar
        \item[-] Unfamiliar
        \item[-] Have some idea
        \item[-] Familiar
        \item[-] Very Familiar
    \end{itemize}
    
    % What do you think the device is
    \item[] 
    \item[] Q4/Q7/Q10/Q13/Q16/Q19/Q22/Q25. What do you think the following device is? Even if you don't know, try to guess what this device is. \figref{fig:survey_devices}
    \newline
    (Open text)
    
    % Comfortableness with device
    \item[] 
    \item[] Q5/Q8/Q11/Q14/Q17/Q20/Q23/Q26. How comfortable are you with this device being placed in your bedroom and streaming/recording data? \figref{fig:survey_devices}
    \begin{itemize}
        \setlength{\itemindent}{-0.3in}
        \item[-] Very Uncomfortable
        \item[-] Uncomfortable
        \item[-] Neutral - Neither comfortable nor uncomfortable
        \item[-] Comfortable
        \item[-] Very Comfortable
    \end{itemize}
    
    % Comfort based on collected data
    % \brian{@Akash please update these with the original high res crops}
    \begin{figure*}[!tbp]
    
        \centering
          \subfloat[]{\includegraphics[width=0.25\textwidth]{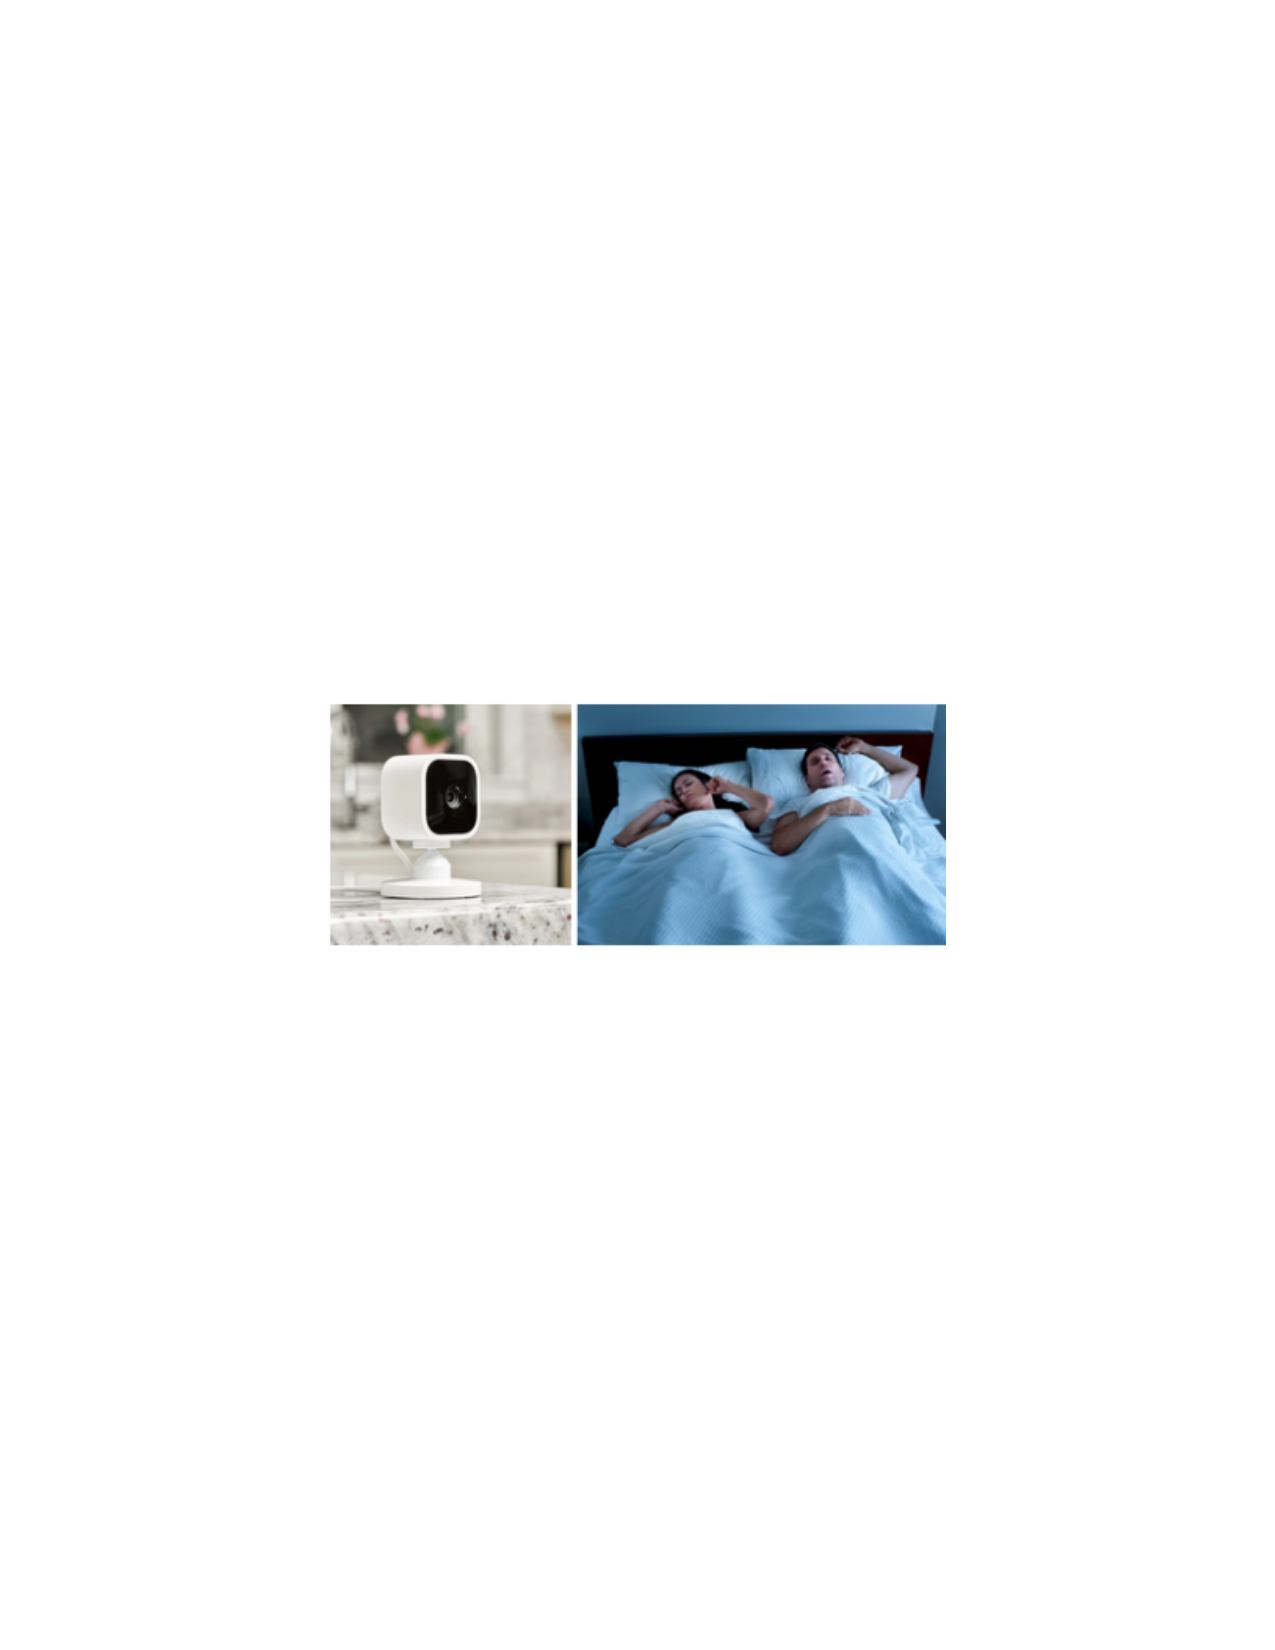}}
         \subfloat[]{\includegraphics[width=0.25\textwidth]{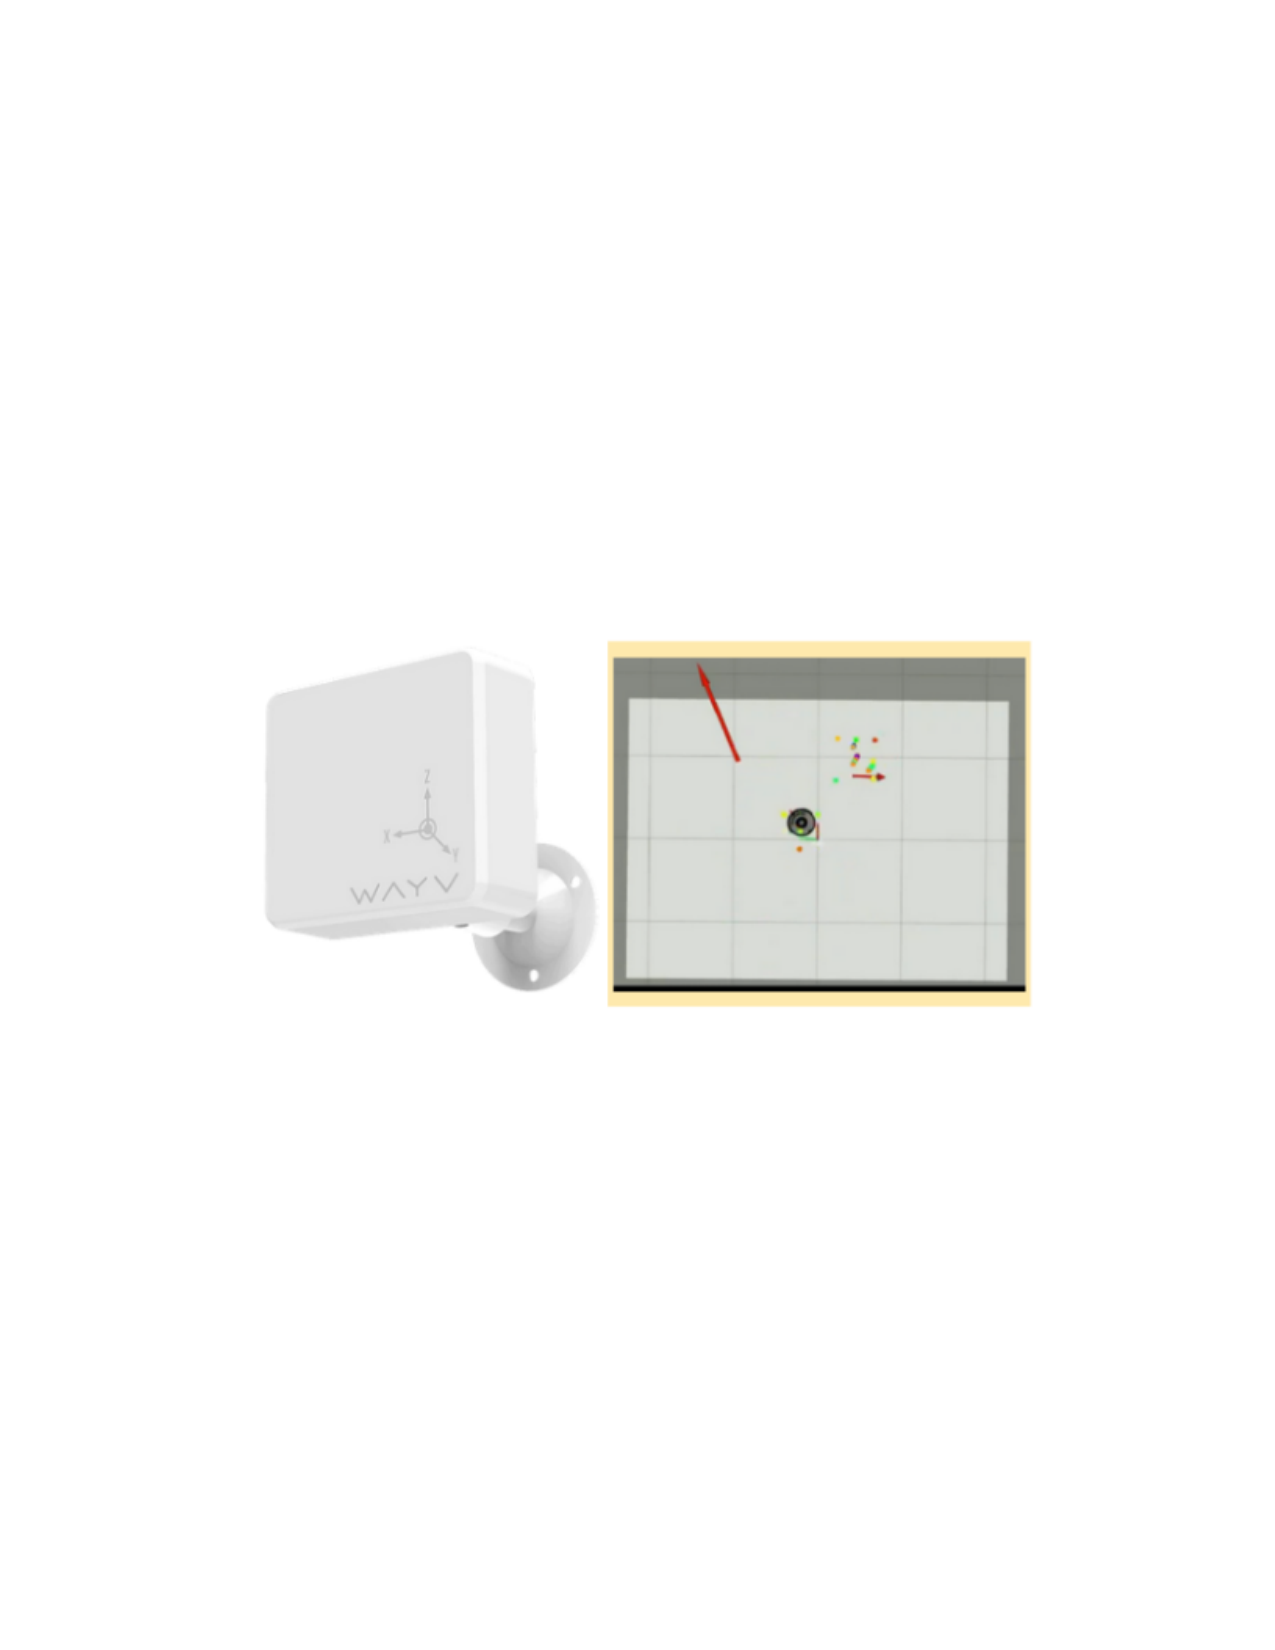}}
         \subfloat[]{\includegraphics[width=0.25\textwidth]{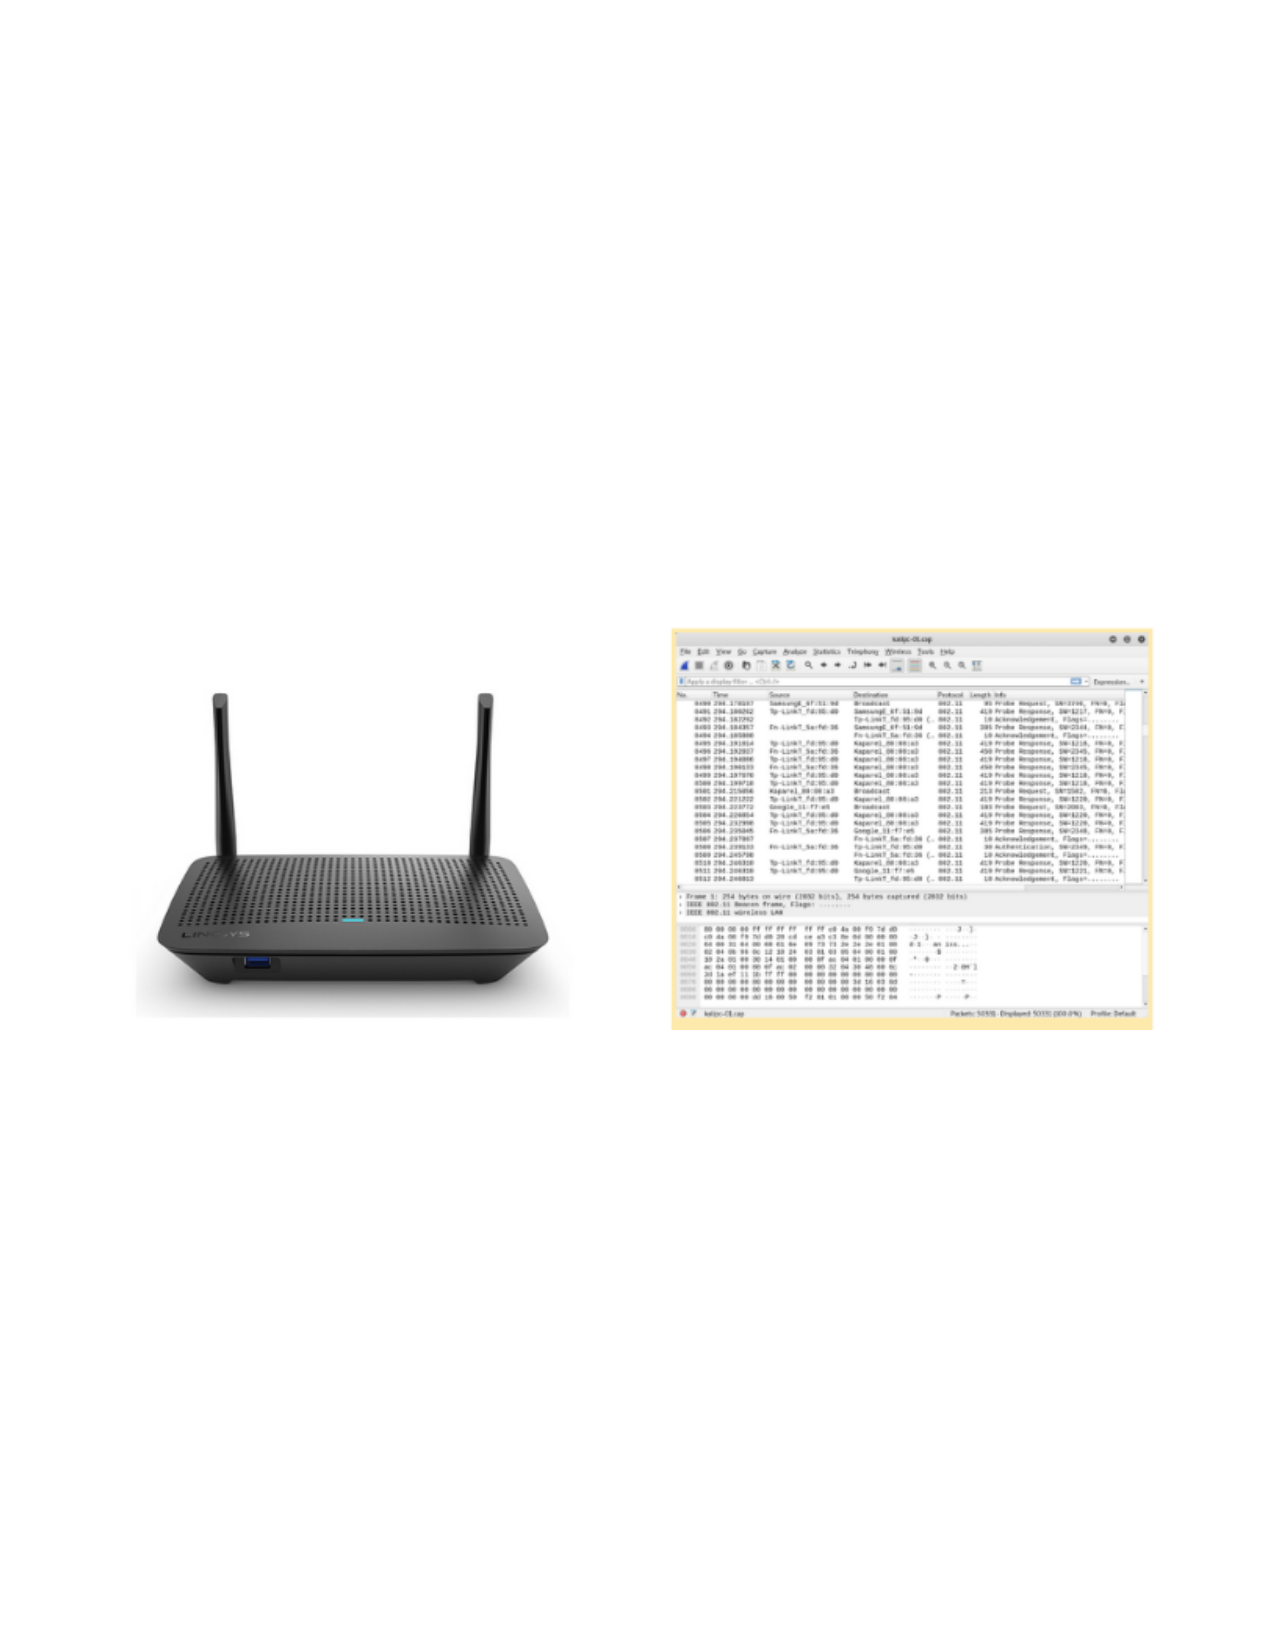}}
       
        \caption{Scenarios involving sensor outputs. (a) Camera and its output image, (b) mmWave radar and its output point-cloud data, and (c) WiFi router and its Wireshark output.}
        \label{fig:collected_data}
    \end{figure*}
    
    \item[] 
    \item[] In the following section, we asked participants to describe their comfort level with respect to a device and the output of its collected data.  This question was asked for each of the 3 scenarios shown in \figref{fig:collected_data}
    
    \item[] 
    \item[] Q27/Q28/Q29. The data collected by the device shown below looks like the rightmost image shown in \figref{fig:collected_data}.  How comfortable are you with this device being placed in your bedroom given the data it collects.
    \begin{itemize}
        \setlength{\itemindent}{-0.3in}
        \item[-] Very Uncomfortable
        \item[-] Uncomfortable
        \item[-] Neutral - Neither comfortable nor uncomfortable
        \item[-] Comfortable
        \item[-] Very Comfortable
    \end{itemize}
    % Describe comfort with inferences
    \item[] In the following section we describe various inferences that can be made by devices, and ask participants how comfortable they are with those inferences being made.
    \item[] 
    \item[] Q30. The device shown in Fig. 8a has a sensor and is from a company that promises that no humans look at the raw sensor data captured by these devices, and that instead only specific outputs produced by algorithms processing the data are shared. The algorithms can make the following inferences about your activities, behaviors, and surroundings:  (i) The number of people (including you) in the room that you are in, and their clothing, race, ethnicity, body shape, height, and posture; (ii) Certain activities, behaviors, and health conditions of the people: having meals, drinking, smoking, walking, praying, watching TV, using a smartphone, intimate moments (hugging, kissing), and breathing rate. How comfortable are you with such a device being placed in your bedroom and sharing the inferences shown above?
    \begin{itemize}
        \setlength{\itemindent}{-0.3in}
        \item[-] Very Uncomfortable
        \item[-] Uncomfortable
        \item[-] Neutral - Neither comfortable nor uncomfortable
        \item[-] Comfortable
        \item[-] Very Comfortable
    \end{itemize}
    \vspace{-0.15in}
     \item[] 
    \item[] Q31. The device shown in Fig. 8b has a sensor and is from a company that promises that no humans look at the raw sensor data captured by these devices, and that instead only specific outputs produced by algorithms processing the data are shared. The algorithms can make the following inferences about your activities, behaviors, and surroundings:  (i) The number of people (including you) in the room that you are in, and their, body shape, height, and posture; (ii) Certain activities, behaviors, and health conditions of the people: having meals, drinking, smoking, walking, praying, watching TV, using a smartphone, intimate moments (hugging, kissing), and breathing rate. How comfortable are you with such a device being placed in your bedroom and sharing the inferences shown above?
    \begin{itemize}
        \setlength{\itemindent}{-0.3in}
        \item[-] Very Uncomfortable
        \item[-] Uncomfortable
        \item[-] Neutral - Neither comfortable nor uncomfortable
        \item[-] Comfortable
        \item[-] Very Comfortable
    \end{itemize}
    \vspace{-0.15in}
     \item[] 
    \item[] Q32. The device shown in Fig. 8c has a sensor and is from a company that promises that no humans look at the raw sensor data captured by these devices, and that instead only specific outputs produced by algorithms processing the data are shared. The algorithms can make the following inferences about your activities, behaviors, and surroundings:  (i) Websites that you’re browsing, total time spent on your smartphone, and sleep schedule; (ii) The number of people (including you) in the room that you are in, and their, body shape, height, and posture; (iii) Certain activities, behaviors, and health conditions of the people: having meals, walking, praying, watching TV, using a smartphone, intimate moments (hugging, kissing), and breathing rate. How comfortable are you with such a device being placed in your bedroom and sharing the inferences shown above?
    \begin{itemize}
        \setlength{\itemindent}{-0.3in}
        \item[-] Very Uncomfortable
        \item[-] Uncomfortable
        \item[-] Neutral - Neither comfortable nor uncomfortable
        \item[-] Comfortable
        \item[-] Very Comfortable
    \end{itemize}
    
    % Scenarios relating to development of devices
     \item[] In the following section, we ask participants about various scenarios.
     \item[] 
    \item[] Q33. Suppose you create your own camera from scratch. You control what the camera looks like, what parts go inside it, what data it collects, and where the data is stored. How comfortable would you be with that camera being placed in your bedroom given that no one else can see the data except you?
    \begin{itemize}
        \setlength{\itemindent}{-0.3in}
        \item[-] Very Uncomfortable
        \item[-] Uncomfortable
        \item[-] Neutral - Neither comfortable nor uncomfortable
        \item[-] Comfortable
        \item[-] Very Comfortable
    \end{itemize}
    
     \item[] 
    \item[] Q34. Please explain the choice you made in the previous question briefly
    \newline
    (Open Text)
    
     \item[] 
    \item[] Q35. Which of the following cameras will you prefer if you have to place one inside your home?
    \begin{itemize}
        \setlength{\itemindent}{-0.3in}
        \item[-] A camera from a well-known brand that does not sell ads or ad revenue is not a major revenue source for them
        \item[-] A camera from a company whose main source of income is ad revenue and sells your data to advertisers
        \item[-] A camera from a company based in the USA
        \item[-] A camera from a company based in a country that you do not trust
    \end{itemize}
    
     \item[] 
    \item[] Q36. Please explain the choice you made in the previous question briefly
    \newline
    (Open Text)

    \item[] In the following section we described a list of various inferences, and asked participants their comfort level for each inference being made.
    \item[] 
    \item[] Q37-Q44. For the following inference about your life inside your house, please assign it a comfort score [From very uncomfortable to very comfortable] based on how comfortable you will be with placing a device in your bedroom that can record/stream that information: 
    \begin{itemize}
        \item Knowledge about and timing of activities being done – walking, sitting on a couch, sleeping, cooking, bathing, working out, etc.
        \item Videos of the activities being done – walking, sitting on a couch, sleeping, cooking, bathing
        \item Your vital signs – heart rate, breathing rate
        \item Your location within your home
        \item When you are using your laptop or smartphone or TV
        \item What kind of content you are watching on your laptop or smartphone or TV – video, audio, web browsing, etc.
        \item Video of the content you are watching on your laptop or smartphone – video, audio, web browsing, etc.
        \item Your daily schedule – when you wake up, sleep, take a shower, watch TV, etc.
    \end{itemize}

\end{itemize}
\endgroup
